# Supplementary material for: Strange Metals from Melting Correlated Insulators in Twisted Bilayer Graphene
Source: arXiv:2105.08069 ancillary file (2021-12-23)
Supplement: Supplementary file 1 [file SI.pdf]

# Supplementary Information for "Strange Metals from Melting Correlated Insulators in Twisted Bilayer Graphene"

Peter Cha,[1] Aavishkar A. Patel,[2] and Eun-Ah Kim[1]

[1]*Department of Physics, Cornell University, Ithaca, New York 14853, USA*
[2]*Department of Physics, University of California, Berkeley, CA 94720, USA*

## I. ALTERNATIVE DERIVATION OF THE EFFECTIVE HAMILTONIAN

We provide an alternate derivation of (2) of the main text. In each hexagonal region $\hexagon$ of area $A_{\hexagon}$ centered at $\mathbf{r}_i$ of Fig. 2a of the main text, we coarse-grain by defining averaged fermion fields $\bar{\Psi}(\mathbf{r}_i)$ as

$$\frac{1}{A_{\hexagon}}\int_{\hexagon} d^2\mathbf{r}\ \Psi^\dagger(\mathbf{r})M^\alpha\Psi(\mathbf{r}) = \int \frac{d^2\mathbf{k}}{(2\pi)^2}\ \Psi^\dagger(\mathbf{r}_i,\mathbf{k})M^\alpha\Psi(\mathbf{r}_i,\mathbf{k}) \equiv \bar{\Psi}^\dagger(\mathbf{r}_i)M^\alpha\bar{\Psi}(\mathbf{r}_i). \tag{1}$$

The definition of the averaged fields $\bar{\Psi}(\mathbf{r}_i)$ therefore absorbs the effects of higher momentum modes and higher bands (which are just higher momentum modes in an unfolded Brillouin zone scheme). Interaction terms, which are quartic in the fermion fields, and have a generic form of

$$H_U \sim \sum_{\alpha,\beta}\int d^2\mathbf{r}d^2\mathbf{r}'C_{\alpha\beta}(\mathbf{r},\mathbf{r}')\Psi^\dagger(\mathbf{r})M^\alpha\Psi(\mathbf{r})\Psi^\dagger(\mathbf{r}')M^\beta\Psi(\mathbf{r}'), \tag{2}$$

can then be decomposed in a mean field fashion and coarse-grained in terms of $\mathcal{O}^\alpha(\mathbf{r}_i) \equiv \langle\bar{\Psi}^\dagger(\mathbf{r}_i)M^\alpha\bar{\Psi}(\mathbf{r}_i)\rangle$, as in many earlier works [1–8], where a mean field wavefunction with a nonzero and spatially uniform value of $\mathcal{O}^\alpha(\mathbf{r}_i)$ leads to an insulating ground state. Within the space of mean field wavefunctions, if the order parameter $\mathcal{O}^\alpha(\mathbf{r}_i)$ is allowed to vary in space, then the decomposed interaction term $H_U$ naturally leads to a Hamiltonian of the form of (2) of the main text, which is Ising-like in the mean field space of states where $M^\alpha$ is a (normalized) Dirac mass matrix with eigenvalues $\pm1$ and the quantization axis $\alpha$ of $M^\alpha$ is taken to be fixed, as in our work.

Physically, the energy cost of spatial fluctuations of $\mathcal{O}(\mathbf{r}_i)$ arises from boundary effects between regions where it takes on different values. For instance, as is well known, a Dirac fermion system with a spatially varying mass term has edge modes that occur on the boundaries of regions with positive and negative masses [9], which affect the ground state energetics (Fig. 1). Since the correlated insulator ground state is expected to be ordered with a spatially uniform $\mathcal{O}(\mathbf{r}_i)$, we choose the coupling constants in (2) of the main text appropriately to achieve this. Since our picture is one of an effective Hamiltonian or effective field theory, the coupling constants $U_{ij}$ of (2) of the main text implicitly contain information about the structure of the various high-energy modes of the microscopic Hamiltonian. However, the precise form of the microscopics is not important to us and we instead look at experimental observations to deduce the appropriate form of $U_{ij}$ (or $J_{1,2}$) as in the next section of this Supplementary Information. Note that the length scale $a_f$ is only used for illustrating the coarse-graining scheme, and its absolute value doesn't appear anywhere in our work - it is only implicit in the values of the coupling constants which we deduce from phenomenology.

In this mean-field, coarse-grained decomposition, the quadratic part of the microscopic Hamiltonian becomes one of Dirac fermions within the $\hexagon$ regions centered at $\mathbf{r}_i$, with a mass gap set by $|\mathcal{O}^\alpha(\mathbf{r}_i)|$. Since the ground-state energy of such a quadratic Hamiltonian is the same whether $\mathcal{O}(\mathbf{r}_i)$ is $+1$ or $-1$ in the Ising case (or, in the case where the quantization axis $\alpha$ of $M^\alpha$ is also allowed to vary in space, independent of the direction of the $\alpha$-vector $\mathcal{O}^\alpha(\mathbf{r}_i)$ as long as its magnitude is fixed), the $\mathcal{O}$ fluctuations considered in our work do not affect the energy of the quadratic part.

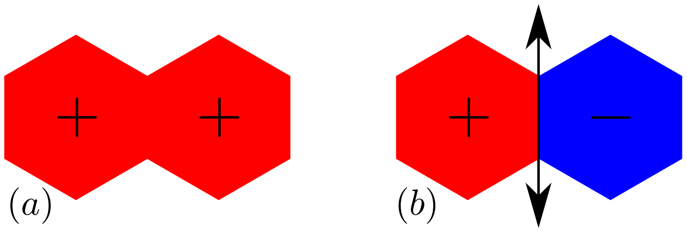


FIG. 1. Between regions with different values of $\mathcal{O}(\mathbf{r}_i)$ (b), there are boundary states that change the total energy of the configuration, which are not present in the homogenous case (a).

Therefore, we do not need to explicitly consider this part of the Hamiltonian in our effective Hamiltonian (2) of the main text, as it is just a fixed energy cost on the manifold of mean field states we consider, even though its *absolute magnitude* may be comparable to that of the interacting part of the Hamiltonian.

The quadratic part of the microscopic Dirac fermion Hamiltonian is important, however, for defining the coarse-grained current operator, which represents the average current in a ⬡ region. It is given by

$$\frac{1}{A_{\hexagon}}\int_{\hexagon} d^2\mathbf{r}\ ev_D^m \Psi^\dagger(\mathbf{r})\Sigma_{x,y}\Psi(\mathbf{r}) = \int \frac{d^2\mathbf{k}}{(2\pi)^2}\ ev_D^m \Psi^\dagger(\mathbf{r}_i,\mathbf{k})\Sigma_{x,y}\Psi(\mathbf{r}_i,\mathbf{k}) \equiv ev_D^m \bar{\Psi}^\dagger(\mathbf{r}_i)\Sigma_{x,y}\bar{\Psi}(\mathbf{r}_i),$$
$$\mathcal{X}(\mathbf{r}_i) \equiv \bar{\Psi}^\dagger(\mathbf{r}_i)\Sigma_x\bar{\Psi}(\mathbf{r}_i), \quad \mathcal{Y}(\mathbf{r}_i) \equiv \bar{\Psi}^\dagger(\mathbf{r}_i)\Sigma_y\bar{\Psi}(\mathbf{r}_i), \tag{3}$$

where $\Sigma_{x,y}$ are the Dirac dispersion/current matrices in the $x, y$ directions respectively, which anticommute with $M^\alpha$, as $M^\alpha$ must open a Dirac mass gap. We can therefore see that the action of $\mathcal{X}(\mathbf{r}_i)$ or $\mathcal{Y}(\mathbf{r}_i)$ on a mean-field state flips the sign of $\mathcal{O}^\alpha(\mathbf{r}_i)$, which allows for the calculation of the conductivity using (5) of the main text.

If we go beyond considering the mean-field space of states that are product states of eigenstates of $\bar{\Psi}^\dagger(\mathbf{r}_i)M^\alpha\bar{\Psi}(\mathbf{r}_i)$, at each $\mathbf{r}_i$, then it is possible to consider the effects of quantum fluctuations beyond the classical description. Such quantum fluctuations may be important in cases where the ordering into the correlated insulator phase is suppressed, but unconventional transport is still observed [10]; the suppression of the Dirac mass will naturally lead to the suppression of $J_1$ and $J_2$ that arise from boundary effects between regions with different signs of the mass, as the distinction between such regions is smaller when the magnitude of the mass is smaller. This would then lead to quantum fluctuations of the order-parameter playing a more significant role in the finite-temperature dynamics. While it is not possible to directly add a transverse-field term coupling to $\mathcal{X}(\mathbf{r}_i)$ or $\mathcal{Y}(\mathbf{r}_i)$ to the Hamiltonian, as that would break inversion and time-reversal symmetries due to these being current operators, one can add terms that couple currents in neighboring regions, leading to models of the quantum XXZ kind instead of the classical Ising kind. Such models may be studied using more advanced numerical techniques than those employed in this work, and will be the focus of future work on this topic.

Finally, if we move away from the integer fillings considered in this work by doping the massive Dirac cones with a chemical potential, there will still be boundary effects between regions with different Dirac masses. We then expect our description of the effective Hamiltonian (2) of the main text to still hold, and the parameters $J_{1,2}$ to smoothly change as a function of the chemical potential. However, as described in the main text, we would now also expect a contribution to the current operator coming from the low-energy quasiparticle excitations near the Fermi surface, in addition to the average current considered in this work. In order to take both contributions into account, we could consider a model with doped massive Dirac cones coupled to the fluctuating mass field $\mathcal{O}^\alpha(\mathbf{r}_i)$, which also self-interacts according to an Ising or XXZ Hamiltonian. The analysis of such fermion-boson models typically requires sophisticated determinantal quantum Monte Carlo simulations [11, 12] that are beyond the scope of this work, but which will be considered in future work. However, we would expect that the Fermi surface will be washed out at higher temperatures due to strong quasiparticle scattering, and therefore its contribution to the conductivity could then become smaller compared to the contribution from the fluctuations of $\mathcal{O}^\alpha(\mathbf{r}_i)$, which would lead to the mechanism studied in this work being applicable at higher temperatures even away from integer fillings.

## II. PARAMETERS AND EXPERIMENTAL ENERGY SCALES

In this section, we will relate the values of the phenomenological parameters $J_{1,2}$ in our model to experimentally observed energy scales. Our classical Monte Carlo simulations in the main text show that the effective Ising model orders into the correlated insulator state at $T \sim J_1$, displaying an upturn in the resistivity. Experimental data [13, 14] features a resistivity upturn at $T \sim 5 - 10$ K. We therefore conclude that this sets the appropriate scale for $J_1$. This temperature scale is much smaller than the order $\sim$ 10 meV (100 K) scale of the Dirac mass band gap at integer fillings, which is measured by scanning tunneling microscopy techniques [15, 16]. This is not surprising in our picture, because $J_{1,2}$ arise from boundary effects between regions where the correlated insulator order-parameter takes on different values, instead of directly from the bulk band gap itself. In fact, this difference between the insulating energy scale in transport measurements at integer fillings and the quasiparticle band gap therefore points to strong correlation effects being responsible for the unconventional transport properties, rather than simply thermally excited quasiparticles being scattered off of phonons.

Since there is a large separation of scales between $J_{1,2}$ and the band gap, as well as between $J_{1,2}$ and the bandwidths and gaps to higher bands, we can safely study transport described by the mechanism in this work over a range of

temperatures, without worrying about exciting high-energy quasiparticles.

---


[1] M. Xie and A. H. MacDonald, Nature of the correlated insulator states in twisted bilayer graphene, Phys. Rev. Lett. **124**, 097601 (2020).

[2] Y.-H. Zhang, D. Mao, and T. Senthil, Twisted bilayer graphene aligned with hexagonal boron nitride: Anomalous Hall effect and a lattice model, Phys. Rev. Research **1**, 033126 (2019).

[3] N. Bultinck, S. Chatterjee, and M. P. Zaletel, Mechanism for anomalous Hall ferromagnetism in twisted bilayer graphene, Phys. Rev. Lett. **124**, 166601 (2020).

[4] S. Liu, E. Khalaf, J. Y. Lee, and A. Vishwanath, Nematic topological semimetal and insulator in magic-angle bilayer graphene at charge neutrality, Phys. Rev. Research **3**, 013033 (2021).

[5] A. Thomson and J. Alicea, Recovery of massless Dirac fermions at charge neutrality in strongly interacting twisted bilayer graphene with disorder, Phys. Rev. B **103**, 125138 (2021).

[6] N. Bultinck, E. Khalaf, S. Liu, S. Chatterjee, A. Vishwanath, and M. P. Zaletel, Ground state and hidden symmetry of magic-angle graphene at even integer filling, Phys. Rev. X **10**, 031034 (2020).

[7] M. Christos, S. Sachdev, and M. S. Scheurer, Superconductivity, correlated insulators, and wess–zumino–witten terms in twisted bilayer graphene, Proceedings of the National Academy of Sciences 10.1073/pnas.2014691117 (2020).

[8] B. Lian, Z.-D. Song, N. Regnault, D. K. Efetov, A. Yazdani, and B. A. Bernevig, Twisted bilayer graphene IV: Exact insulator ground states and phase diagram, Phys. Rev. B **103**, 205414 (2021).

[9] C. Fosco and A. López, Dirac fermions and domain wall defects in $2+1$ dimensions, Nuclear Physics B **538**, 685 (1999).

[10] A. Jaoui, I. Das, G. Di Battista, J. Díez-Mérida, X. Lu, K. Watanabe, T. Taniguchi, H. Ishizuka, L. Levitov, and D. K. Efetov, Quantum-critical continuum in magic-angle twisted bilayer graphene, arXiv preprint arXiv:2108.07753 (2021).

[11] Y. Schattner, S. Lederer, S. A. Kivelson, and E. Berg, Ising nematic quantum critical point in a metal: A Monte Carlo study, Phys. Rev. X **6**, 031028 (2016).

[12] X. Y. Xu, K. Sun, Y. Schattner, E. Berg, and Z. Y. Meng, Non-Fermi liquid at $(2+1)$D ferromagnetic quantum critical point, Phys. Rev. X **7**, 031058 (2017).

[13] Y. Cao, D. Chowdhury, D. Rodan-Legrain, O. Rubies-Bigorda, K. Watanabe, T. Taniguchi, T. Senthil, and P. Jarillo-Herrero, Strange metal in magic-angle graphene with near Planckian dissipation, Phys. Rev. Lett. **124**, 076801 (2020).

[14] J. M. Park, Y. Cao, K. Watanabe, T. Taniguchi, and P. Jarillo-Herrero, Flavour Hund's coupling, Chern gaps and charge diffusivity in Moiré graphene, Nature **592**, 43 (2021).

[15] Y. Xie, B. Lian, B. Jäck, X. Liu, C.-L. Chiu, K. Watanabe, T. Taniguchi, B. A. Bernevig, and A. Yazdani, Spectroscopic signatures of many-body correlations in magic-angle twisted bilayer graphene, Nature **572**, 101 (2019).

[16] K. P. Nuckolls, M. Oh, D. Wong, B. Lian, K. Watanabe, T. Taniguchi, B. A. Bernevig, and A. Yazdani, Strongly correlated Chern insulators in magic-angle twisted bilayer graphene, Nature **588**, 610 (2020).
